# Supplementary material for: Comparing the Effects of DNS, DoT, and DoH on Web Performance
Source: arXiv:1907.08089 source file (2020-02-23)
Supplement: Supplementary file 1 [file appendix.tex]

\section{Appendix}
\begin{table*}[t!]
  \centering
  \footnotesize
  \rowcolors{1}{}{lightgray}
  
  \begin{tabularx}{\textwidth}{Xlrrrrrrrrrr}
    & & \textbf{Default} & \multicolumn{3}{c}{\textbf{Quad9}} & \multicolumn{3}{c}{\textbf{Google}} & \multicolumn{3}{c}{\textbf{Cloudflare}}\\
    \rowcolor{black}\cline{3-12}
    \rowcolor{white}\textbf{Connectivity} & \textbf{Status} & Do53 & Do53 & DoT & DoH & Do53 & DoT & DoH & Do53 & DoT & DoH\\
    \arrayrulecolor{black}\hline
      \cellcolor{white}
        & Successful
        & 76.11\%
        & 76.29\%
        & 75.53\%
        & 73.65\%
        & 76.08\%
        & 75.51\%
        & 74.63\%
        & 76.39\%
        & 76.24\%
        & 75.13\%
        \\
      \cellcolor{white}
        & Page-load Timeout
        & 9.77\%
        & 9.61\%
        & 10.05\%
        & 9.18\%
        & 9.95\%
        & 9.83\%
        & 9.63\%
        & 9.71\%
        & 9.70\%
        & 9.47\%
        \\
      \cellcolor{white}
        & DNS Error
        & 9.44\%
        & 9.46\%
        & 9.43\%
        & 10.57\%
        & 9.29\%
        & 9.28\%
        & 9.72\%
        & 9.32\%
        & 9.27\%
        & 9.42\%
        \\
      \cellcolor{white}
        & Selenium Error
        & 1.84\%
        & 1.83\%
        & 1.89\%
        & 1.74\%
        & 1.86\%
        & 1.89\%
        & 1.86\%
        & 1.86\%
        & 1.86\%
        & 1.79\%
        \\
      \cellcolor{white}\multirow{-5}{*}{Default network}
        & Other Error
        & 4.68\%
        & 4.64\%
        & 4.99\%
        & 6.60\%
        & 4.68\%
        & 5.38\%
        & 6.02\%
        & 4.58\%
        & 4.79\%
        & 5.98\%
        \\
    \arrayrulecolor{gray}\hline
    \cellcolor{lightgray}
        & Successful
        & 76.59\%
        & 76.92\%
        & 76.32\%
        & 75.08\%
        & 76.91\%
        & 77.43\%
        & 76.55\%
        & 77.18\%
        & 77.58\%
        & 77.48\%
        \\
      \cellcolor{lightgray}
        & Page-load Timeout
        & 10.49\%
        & 10.53\%
        & 11.23\%
        & 10.14\%
        & 10.47\%
        & 10.55\%
        & 10.44\%
        & 10.59\%
        & 10.33\%
        & 10.23\%
        \\
      \cellcolor{lightgray}
        & DNS Error
        & 9.37\%
        & 9.46\%
        & 9.47\%
        & 11.63\%
        & 9.27\%
        & 9.28\%
        & 10.09\%
        & 9.30\%
        & 9.29\%
        & 9.51\%
        \\
      \cellcolor{lightgray}
        & Selenium Error
        & 1.86\%
        & 1.88\%
        & 1.85\%
        & 1.79\%
        & 1.80\%
        & 1.72\%
        & 1.82\%
        & 1.74\%
        & 1.86\%
        & 1.84\%
        \\
      \cellcolor{lightgray}\multirow{-5}{*}{4G network}
        & Other Error
        & 3.55\%
        & 3.09\%
        & 2.98\%
        & 3.15\%
        & 3.35\%
        & 2.74\%
        & 2.92\%
        & 2.93\%
        & 2.80\%
        & 2.78\%
        \\
    \arrayrulecolor{gray}\hline
    \cellcolor{white}
        & Successful
        & 77.42\%
        & 77.10\%
        & 76.65\%
        & 75.18\%
        & 77.18\%
        & 77.59\%
        & 76.24\%
        & 76.97\%
        & 77.92\%
        & 77.89\%
        \\
      \cellcolor{white}
        & Page-load Timeout
        & 10.42\%
        & 10.74\%
        & 11.19\%
        & 9.46\%
        & 10.65\%
        & 10.48\%
        & 10.40\%
        & 10.52\%
        & 10.23\%
        & 9.98\%
        \\
      \cellcolor{white}
        & DNS Error
        & 9.36\%
        & 9.39\%
        & 9.42\%
        & 12.16\%
        & 9.23\%
        & 9.23\%
        & 10.47\%
        & 9.29\%
        & 9.25\%
        & 9.50\%
        \\
      \cellcolor{white}
        & Selenium Error
        & 1.81\%
        & 1.60\%
        & 1.71\%
        & 1.89\%
        & 1.71\%
        & 1.76\%
        & 1.87\%
        & 1.71\%
        & 1.72\%
        & 1.69\%
        \\
      \cellcolor{white}\multirow{-5}{*}{Lossy 4G network}
        & Other Error
        & 2.80\%
        & 2.77\%
        & 2.74\%
        & 3.20\%
        & 2.94\%
        & 2.70\%
        & 2.89\%
        & 3.22\%
        & 2.60\%
        & 2.63\%
        \\
    \arrayrulecolor{gray}\hline
    \cellcolor{lightgray}
        & Successful
        & 22.65\%
        & 22.29\%
        & 22.13\%
        & 9.86\%
        & 22.45\%
        & 22.67\%
        & 13.66\%
        & 22.46\%
        & 22.42\%
        & 17.62\%
        \\
      \cellcolor{lightgray}
        & Page-load Timeout
        & 66.21\%
        & 66.50\%
        & 66.54\%
        & 29.02\%
        & 66.46\%
        & 66.02\%
        & 40.63\%
        & 66.40\%
        & 66.51\%
        & 51.40\%
        \\
      \cellcolor{lightgray}
        & DNS Error
        & 9.32\%
        & 9.39\%
        & 9.50\%
        & 60.11\%
        & 9.23\%
        & 9.32\%
        & 44.39\%
        & 9.25\%
        & 9.25\%
        & 29.48\%
        \\
      \cellcolor{lightgray}
        & Selenium Error
        & 1.48\%
        & 1.53\%
        & 1.56\%
        & 0.65\%
        & 1.55\%
        & 1.70\%
        & 0.95\%
        & 1.59\%
        & 1.51\%
        & 1.22\%
        \\
      \cellcolor{lightgray}\multirow{-5}{*}{3G network}
        & Other Error
        & 1.82\%
        & 1.82\%
        & 1.83\%
        & 1.01\%
        & 1.86\%
        & 1.99\%
        & 1.32\%
        & 1.89\%
        & 1.82\%
        & 1.50\%
        \\
    \arrayrulecolor{black}\hline
  \end{tabularx}
  \caption{Successful website page-loads and error percentages for different network conditions.}
  \label{tab:failure}
\end{table*}

\subsection{Error Table for All Providers}\label{app:errortable}
\noindent
Please see \Fref{tab:failure}.
